# Supplementary material for: Intermittent Run Motility of Bacteria in Gels Exhibits Power-Law Distributed Dwell Times
Source: arXiv:2408.02317 source file (2024-08-05)
Supplement: Supplementary file 1 [file Supplement.pdf]

# SUPPLEMENTAL MATERIAL
## Intermittent Run Motility of Bacteria in Gels Exhibits Power-Law Distributed Dwell Times

Agniva Datta, Sönke Beier, Veronika Pfeifer, Robert Großmann, and Carsten Beta

## I. CELL PREPARATION

The strain *P. putida* KT2440 $\text{FliC}_{\text{S267C}}$ was used in this study. The introduction of a surface-exposed cysteine residue in the flagellar subunit FliC enables fluorescent staining of the flagella without a negative effect on swimming motility. Therefore, we refer to this strain as the wild type. Additionally the *P. putida* KT2440 $\text{FliC}_{\text{S267C}}$ $\Delta motAB$ and $\Delta motCD$ mutant strains were used to study the swimming motility in agar. The $\Delta motAB$ and $\Delta motCD$ stator mutants were generated in Ref. [1]. The strains were grown overnight in LB media as a shaking culture at 30 °C in all experiments except for fluorescent staining experiments where tryptone broth (10 g/L tryptone [Applichem], 5 g/L NaCl) was used. Flagellar staining was performed according to Ref. [2] using the fluorescent dye Alexa 488 $C_5$ maleimide (Thermo Fisher Scientific). Additionally, the cell body was stained by adding 10 µl FM 4-64 (Thermo Fisher Scientific; 1 µg/µl in dimethyl sulfoxide) before the final washing step. Semisolid agar was prepared with 210 mM $Na_2HPO_4$, 220 mM $KH_2PO_4$, 50 mM NaCL, 1 mM $MgSO_4$, 0.2 % glucose, 0.5 % casamino acids and 0.25% or 0.3% agar [3]. Agar was poured into FluoroDish cell culture dishes with glass bottoms. After 4 hours for solidification, 2 µl cells at an $\text{OD}_{600\text{nm}}$ of one were injected into the agar. Fluorescence images were recorded after additional four hours. Phase contrast recordings were done at the next day when cells spread circularly from the injection point.

## II. MICROSCOPY

Microscopy was performed in agar at the edge of the spreading culture using an inverted microscope (Olympus IX71) with a high-speed camera (Orca-Fusion BT digital CMOS camera, Hamamatsu) and the Hokawo software (Hamamatsu). Phase contrast recordings were taken 30 µm above the bottom surface with a 20x objective (UPLFLN-PH, Olympus) for 60 seconds at a frame rate of 20 frames per second. Fluorescence images were made close to the bottom surface with a 60x objective (UPLFLN-PH, Olympus) for 10 seconds at a frame rate of 100 frames per second. To separate the cell body from the flagellar fluorescent signal, the W-View Gemini image splitting optics (Hamamatsu) was added to the microscopy setup.

## III. ANALYSIS OF TRAJECTORIES

In this section, we show how model parameters were obtained from experimental data and, in addition, discuss the criterion which was used to identify run episodes. We show the results for all the three cell lines of *P. putida* in 0.25 % agar (wild type, $\Delta motAB$ and $\Delta motCD$).

### A. Cell tracking

To perform segmentation and cell tracking, we used the method described in Ref. [4], which is based on Ref. [5].

### B. Distinction of runs and events

In order to distinguish between the run phases and the immobile phases (events) in the recorded trajectories, at first we used the method proposed in Ref. [6]: a speed threshold was used to distinguish between run and event phases. We have set this threshold to 7 µm/s (a little bit lower then the half of the slowest swimming wrapped mode in bulk [2]). We labeled all data points with a speed under 7 µm/s as events. Fig. S1A reveals that this criterion is not sufficient to detect the events. Oftentimes, one true events is broken down into several smaller events, which are interrupted by short runs. This is because, in between the trap events, the bacteria often swim back and forth. As a result, the measured speed of a bacterium may be faster than the threshold for a short period of time.

We resolved this problem by setting a minimum distance (2 µm: comparable to the length of the bacterium) between two consecutive events in addition to the speed threshold; two consecutive events which are less than 2 $\mu m$ apart from each other were fused, including all intermediate points of the trajectory. In Fig. S1B it can be seen that this detection works much more reliably on our data. Slightly different speed thresholds had no effect on the quality of the detection.

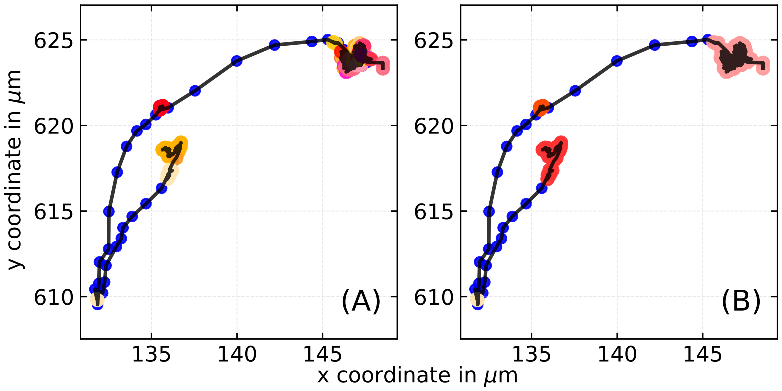


Figure S1. Trajectory comparison: Run phases are marked in blue. The events have different (randomly chosen) colors. (A) Only the velocity threshold of 7 µm/s is used. This leads to a detection of multiple events at a specific cluster of data points which clearly correspond to one event. (B) The minimum distance criterion of 2 µm along with the velocity threshold of 7 µm/s is used. This leads to a fusion of multiple, close by events resulting in a better distinction of runs and events.

We plotted the distributions of the angular changes during runs (by considering the change in direction between the beginning and end of the runs) and that of events (by considering the change in previous run direction compared to that of the next run direction after an event). It can be seen in Fig. S2A that just by the velocity threshold and the minimum distance criterion, we can observe a significant difference in these angular change distributions for runs (peak in zero) and turn events (peak in 180°). However, for the runs, we clearly observe a smaller but significant peak in 180° as well, which clearly indicates that we are missing some short turn events (reversals) which contribute significantly to the overall motility pattern.

To have a more robust and precise run and event distinction, we use an algorithm based on unsupervised machine learning as described in the main text. At first, we smooth the trajectories over 3 data points (moving average). Afterwards, the following characteristics are calculated for each point in a trajectory: change of direction of motion at a given data point for a shorter time interval (one frame), change of direction of motion over a longer time interval (two frames) at that data point, and mean of the speeds incoming and leaving that data point. From a list of potential other observables, we obtained these three characteristics as the most relevant ones for the distinction of runs and events by principle component analysis. Then, we perform a k-means clustering on these three variables in order to distinguish the data points into two distinct categories: run phases and events (turns, stops, traps, reversals). In addition, we use the minimum distance criterion of 2 µm to fuse close by events to obtain the final labels for every data-point in the trajectories in terms of runs and events. It can be seen in Fig. S2B that it not only improves the angular change distribution plots for runs (the peak in 180° disappears, signifying no misdetections) but also does not require the velocity threshold parameter (7 µm/s) that we had to impose for the previous distinction algorithm. We use these labels for further analysis as described below.

We note that trajectories were not smoothed for the analysis of bacterial motility in 0.3 % agar as run times are significantly shorter and runs may be lost by smoothing. Also for the k-means clustering, we consider these three observables to be most relevant by principal component analysis: change of direction of motion at a given data point for a shorter time interval (one frame), change of direction of motion over a longer time interval (four frames) at that data point, and mean of the speeds incoming and leaving that data point.

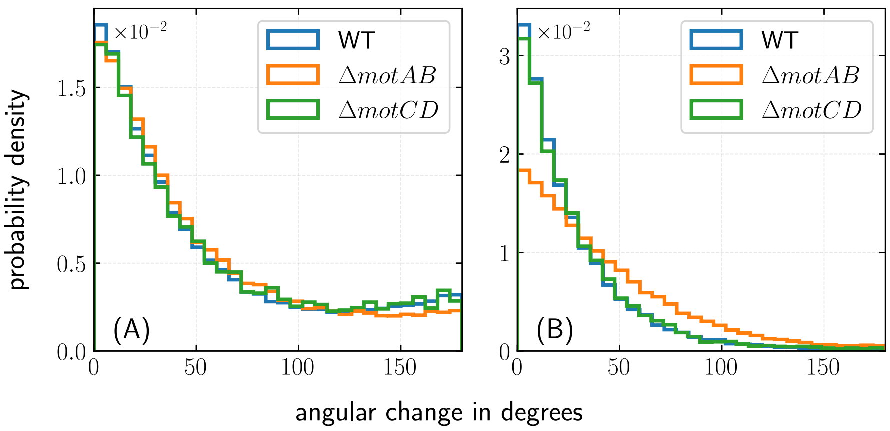


Figure S2. Comparison of angular changes during runs. (A) Distinction algorithm using the minimum distance criterion of 2 µm along with the velocity threshold of 7 µm/s. A small but significant peak at 180° suggests that some short turn events were not detected (particularly reversals). (B) Distinction algorithm using k-means clustering leading to a better distinction where the peak at 180° is absent.

### C. Run time and dwell time distributions

In order to obtain the run time and dwell time statistics in form of survival time probabilities as shown in Fig. 3 in the main text, we classify the data into four categories: both, beginning and end of a phase are observed; only the end of a phase is observed; only the beginning of a phase is observed; neither the beginning nor the end of a phase are observed. Besides the first category, all run times are censored. Then, we apply a non-parametric maximum likelihood approach proposed by Vardi in Ref. [7] to extract the survival time probabilities corresponding to the run time and dwell time distributions.

We fit the survival probability of the run time distribution using the survival function of a double-exponential distribution with a minimum time defined as follows:

$$\psi_R(t) = \begin{cases} 0 & t \leq t_0, \\ p\kappa e^{-\kappa(t-t_0)} + (1-p)\lambda e^{-\lambda(t-t_0)} & t > t_0. \end{cases} \tag{S1}$$

We obtain the parameters $p, \kappa, \lambda, t_0$ from the fit of $\Psi_R\,(t) = \int_t^\infty \psi_R(x)\,dx$. Similarly, we fit the survival probability of the dwell time distribution using the the survival function of a piecewise power law with a minimum time defined as follows:

$$\psi_T(t) = \begin{cases} 0 & t < \tau_1, \\ At^{-\alpha} & t \in (\tau_1, \tau_2), \\ Bt^{-\beta} & t > \tau_2, \end{cases} \tag{S2}$$

where $A = \dfrac{(\alpha-1)\,(\beta-1)\,(\tau_1\tau_2)^\alpha}{(\beta-1)\,\tau_1\tau_2^\alpha + (\alpha-\beta)\,\tau_1^\alpha\tau_2}$ and $B = A{\tau_2}^{\beta-\alpha}$ are chosen such that $\psi_T(t)$ is normalized and continuous. The parameters of this distribution were obtained by fitting the corresponding survival functions $\Psi_T(t) = \int_t^\infty \psi_T(x)\,dx$, shown in Fig. 3 of the main text and Fig. S3.

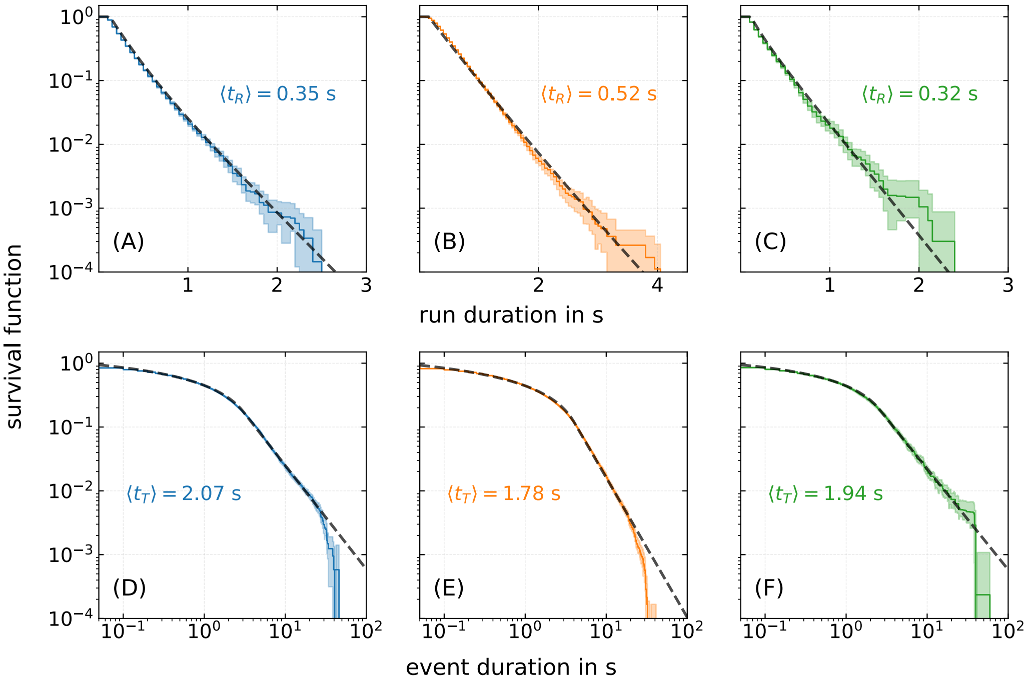


Figure S3. In the top panel (A-C), the survival functions corresponding to the run time distribution $\psi_R(t)$ for *P. putida* wild type (WT), $\Delta motAB$, $\Delta motCD$ along with their respective fits are displayed. In the bottom panel (D-F), the survival functions corresponding to the dwell time distribution $\psi_T(t)$ for wild type, $\Delta motAB$, $\Delta motCD$ along with their respective fits are shown. In all panels, the mean values of the probability distributions are given.

We further computed the mean run time $\langle t_R \rangle$ and the mean dwell time $\langle t_T \rangle$ as shown in Fig. S3 from the expressions of $\psi_R(t)$ and $\psi_T(t)$:

$$\langle t_R \rangle = \int_0^\infty t \cdot \psi_R(t)\, dt = t_0 + \frac{p}{\kappa} + \frac{1-p}{\lambda}, \tag{S3a}$$

$$\langle t_T \rangle = \int_0^\infty t \cdot \psi_T(t)\, dt = \frac{A\left(\tau_2^{2-\alpha} - \tau_1^{2-\alpha}\right)}{2-\alpha} - \frac{B\tau_2^{2-\beta}}{2-\beta}. \tag{S3b}$$

We obtained the mean run time and mean dwell time $(\langle t_R \rangle, \langle t_T \rangle)$ of $(0.35, 2.07)$ s for wild type cells in 0.25 % agar, $(0.23, 3.63)$ s for wild type in 0.3 % agar, as well as $(0.52, 1.78)$ s for $\Delta motAB$ and $(0.32, 1.94)$ s for $\Delta motCD$, both in 0.25 % agar.

### D. Rotational diffusion coefficient $D_\phi$ and tumble parameter $\Gamma$

Experimentally observed runs possess a finite persistence length. Angular fluctuations during run episodes are taken into account in the model via rotational Brownian motion, cf. Eq. (1) in the main text. This implies that the angular change of the direction of motion in between two consecutive frames follows a Gaussian distribution

$$P(\phi, \Delta t) = \frac{1}{\sqrt{4\pi D_\phi \Delta t}} e^{-\frac{\phi^2}{4D_\phi \Delta t}} \tag{S4}$$

with the variance $\langle \phi^2 \rangle = 2D_\phi \Delta t$. We consider all the run-episodes of all trajectories and plot a histogram of the angular changes at each frame. A normal distribution is fitted to the histogram. From the variance of the fitted Gaussian curve, we obtain the rotational diffusion coefficient $D_\phi$. This is illustrated in Fig. S4 for all cell lines.

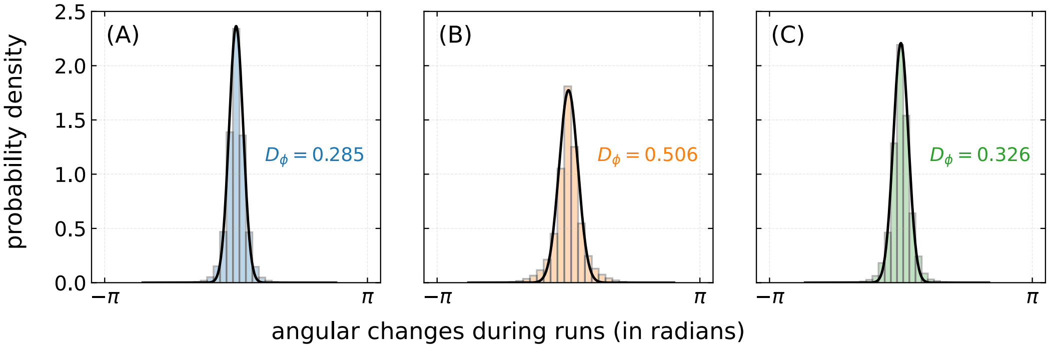


Figure S4. The rotational diffusion coefficient $D_\phi$ is obtained by fitting a normal distribution to the histogram of angular changes during runs for (A) *P. putida* wild type cells (WT), (B) $\Delta motAB$ and (C) $\Delta motCD$. The units of $D_\phi$ as shown are expressed as $s^{-1}$.

The tumble parameter $\Gamma = \langle \cos \Delta\phi \rangle$ is calculated as the mean cosine of the change of direction of motion between two consecutive runs—it is obtained from the distributions shown in Fig. 2A in the main text.

### E. Run speed $v_0$

The run speed parameter $v_0$ can be obtained in many different ways. However, since the MSD curves show a ballistic behaviour universally for all the cell lines for small time lags, we infer it by fitting the ballistic part of the MSD with a power law ($m_2 \sim \Delta^2$); note that the MSD scales with $v_0^2 \Delta^2$ for small time lags $\Delta$ in our model. We verify that the inferred values are consistent with the run speed distribution of bacteria as shown in Fig. S5.

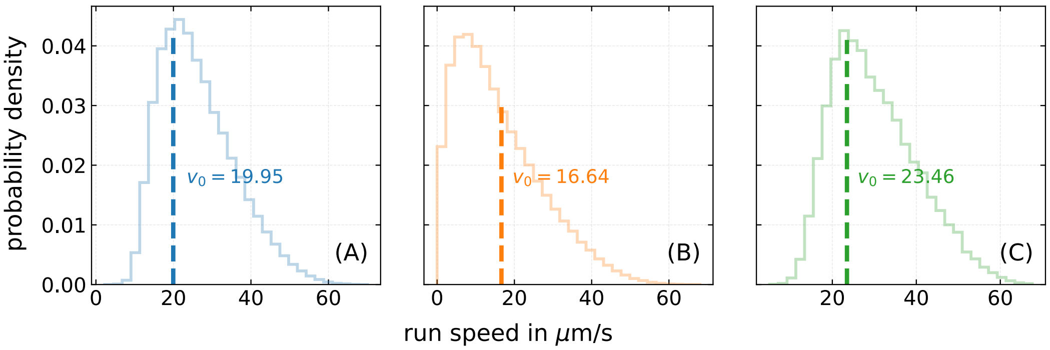


Figure S5. The run speed distribution of (A) *P. putida* wild type (WT), (B) $\Delta motAB$ and (C) $\Delta motCD$. The dotted lines correspond to speed values obtained by fitting the ballistic part of the MSDs (see Fig. 4 in the main text and Fig. S6). The units of $v_0$ as shown are expressed as µm/s.

## IV. MSD AND DIFFUSION COEFFICIENT

We finally plug in all inferred parameters (see Table S1) in the analytical expression of the MSD as stated in Eq. (3) in the main text. Subsequently, a dual inverse Laplace transform is performed numerically to obtain the MSD in time domain and plot it as a function of the lag time $\Delta$ in comparison to the MSD curves obtained from experimental data (Fig. S6). The second temporal variable, which is the aging time $t_a$, is approximated to be one frame—it is a floating parameter that we cannot directly measure from the experiment. We get a very consistent match of our analytical expression of the MSD with the experimentally observed MSD for all cell lines.

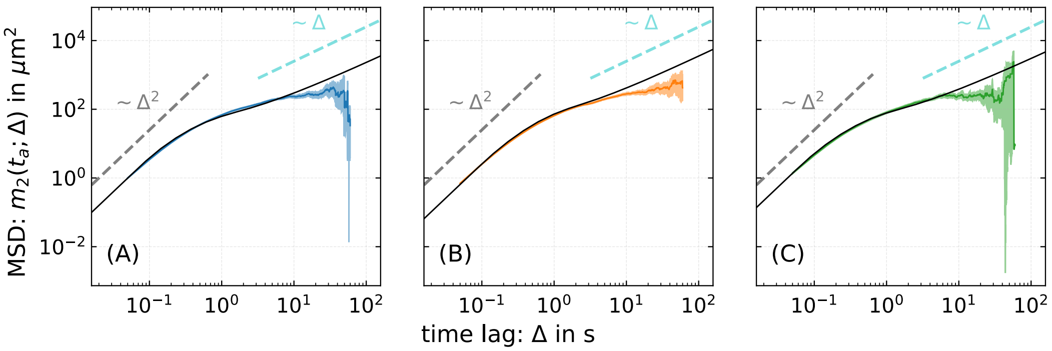


Figure S6. MSD predicted by the model for inferred parameter values, compared to the experimental MSD in color for (A) *P. putida* wild type, (B) $\Delta motAB$ and (C) $\Delta motCD$. The patches correspond to the error bars obtained by bootstrapping.

From Eq. (4) in the main text, we determine the long-term diffusion coefficients by plugging in all the parameters we obtained from the analysis as described in the previous section, summarized in Table S1.

| **cell line** | $v_0$ | $D_\phi$ | $\Gamma = \langle\cos\Delta\phi\rangle$ | $\psi_R$ [Eq. (S1)] | | | | $\psi_T$ [Eq. (S2)] | | | |
|---|---|---|---|---|---|---|---|---|---|---|---|
| | | | | $t_0$ | $\kappa$ | $\lambda$ | $p$ | $\tau_1$ | $\tau_2$ | $\alpha$ | $\beta$ |
| WT | 19.95 | 0.29 | −0.22 | 0.13 | 6.07 | 3.27 | 0.61 | 0.03 | 3.06 | 0.79 | 2.63 |
| $\Delta motAB$ | 16.64 | 0.506 | −0.12 | 0.15 | 3.07 | 2.31 | 0.62 | 0.03 | 4.01 | 0.83 | 3.19 |
| $\Delta motCD$ | 19.95 | 0.29 | −0.22 | 0.12 | 9.77 | 4.00 | 0.29 | 0.03 | 2.56 | 0.75 | 2.58 |

Table S1. The table summarizes all inferred parameter values, obtained from the analysis as described in Section III for *P. putida* cells in 0.25 % agar. Parameters are expressed in the following units: $v_0$ in µm/s; $D_\phi$, $\kappa$ and $\lambda$ in $s^{-1}$; $t_0$, $\tau_1$ and $\tau_2$ in s.

For the wild type cell line in 0.3 % agar, we inferred the following parameter values: $v_0 = 19.49\,\mu m/s$, $D_\phi = 1.33\,s^{-1}$, $\Gamma = -0.25$, $t_0 = 0.08\,s$, $\kappa = 8.04\,s^{-1}$, $\lambda = 3.37\,s^{-1}$, $p = 0.99$, $\tau_1 = 0.02\,s$, $\tau_2 = 3.95\,s$, $\alpha = 0.68$, $\beta = 2.70$. Also, we put the floating parameter $t_a$ to be five frames.

## V. COMPARISON OF RUN LENGTH DISTRIBUTIONS

In this appendix section, we address the differences of run length and run time distributions of the *P. putida* cells in 0.25 % agar. In the main text (Fig. 3), we show and discuss the distribuion of run times. Whereas the statistics of run times of *P. putida* wild type cells and the $\Delta motCD$ mutants cells are practically indistinguishable, we found significantly longer run times of $\Delta motAB$ cells. However, the run speed of $\Delta motAB$ cells is reduced in comparison to the other cell lines as reported earlier in Ref. [1]. That is why we also compared the run length distribution in Fig. S7A—notably, the analysis reveals identical run length distributions for all cell lines. This underlines that the run length of bacteria in agar is not determined by the specifics of cells and their turning behavior, but is rather a consequence of the random structure of the agar matrix.

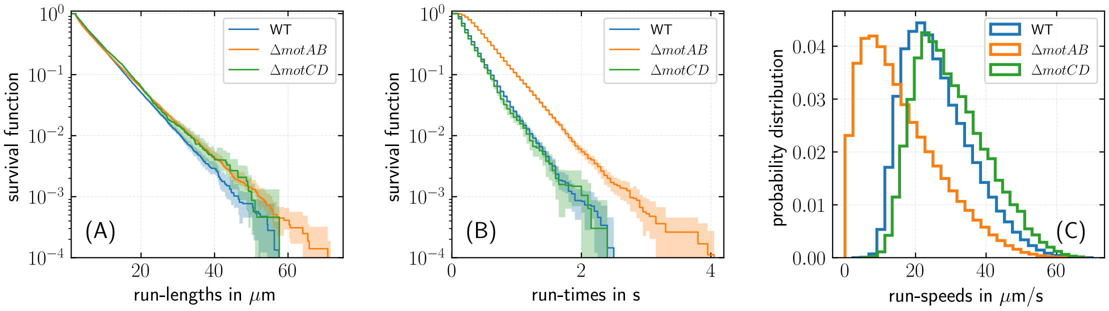


Figure S7. Run length vs. run time distribution of *P. putida* wild type (WT) in blue, $\Delta motAB$ (orange) and $\Delta motCD$ (green) strains in 0.25% agar. (A) Survival function/cumulative probability distribution of run lengths; (B) survival function/cumulative probability distribution of run times; (C) probability density function of run speeds. The patches in panels (A, B) correspond to error bars obtained by bootstrapping.


[1] V. Pfeifer, S. Beier, Z. Alirezaeizanjani, and C. Beta, Role of the two flagellar stators in swimming motility of *Pseudomonas putida*, mBio **13**, 1 (2022).

[2] M. Hintsche, V. Waljor, R. Großmann, M. J. Kühn, K. M. Thormann, F. Peruani, and C. Beta, A polar bundle of flagella can drive bacterial swimming by pushing, pulling, or coiling around the cell body, Sci. Rep. **7**, 16771 (2017).

[3] D.-G. Ha, S. L. Kuchma, and G. A. O'Toole, Plate-based assay for swimming motility in *Pseudomonas aeruginosa*, in *Pseudomonas Methods and Protocols*, Methods in Molecular Biology, Vol. 1149, edited by A. Filloux and J.-L. Ramos (Springer New York, 2014) pp. 59–65.

[4] M. Theves, J. Taktikos, V. Zaburdaev, H. Stark, and C. Beta, A bacterial swimmer with two alternating speeds of propagation, Biophys. J. **105**, 1915 (2013).

[5] J. C. Crocker and D. G. Grier, Methods of digital video microscopy for colloidal studies, J. Colloid Interface Sci. **179**, 298 (1996).

[6] T. Bhattacharjee and S. S. Datta, Bacterial hopping and trapping in porous media, Nat. Commun. **10**, 2075 (2019).

[7] Y. Vardi, Nonparametric estimation in renewal processes, Ann. Stat. **10**, 772 (1982).
